# Supplementary material for: ACES: Generating Diverse Programming Puzzles with with Autotelic Generative Models
Source: arXiv:2310.10692 source file (2024-05-29)
Supplement: Supplementary file 1 [file program_examples_appendix.tex]

\begin{figure}
\begin{python}
def f(ops: List[str], target=2021, nums=[4, 6, 2, 1, 1, 3, 9]):
    assert len(ops) == len(set(ops)) and set(ops) == {"**", "*", "+", "-", "//", "%"}
    expr = str(nums[0])
    for n, op in zip(nums[1:], ops):
        expr += op + str(n)
    return eval(expr) == target

def g(target=2021, nums=[4, 6, 2, 1, 1, 3, 9]):
    """
    Find a permutation of the operators +-*/^
    which when inserted between nums evaluates to target

    target=3, nums=[7, 2, 3, 4, 5, 1, 6] => ["+", "*", "**", "", "//", "-"]
    because 7 + 2 * 3 ** 4 % 5 // 1 - 6 == 3
    """
    from itertools import permutations
    for ops in permutations(["**", "*", "+", "-", "//", "%"]):
        expr = str(nums[0])
        for n, op in zip(nums[1:], ops):
            expr += op + str(n)
        try:
            if eval(expr) == target:
                return list(ops)
        except (ZeroDivisionError, SyntaxError):
            pass
    assert False
assert f(g()) == True

\end{python}

% \end{figure}

% \begin{figure}
\begin{python}

def f(hands: List[int], target_angle=45):
    """Find clock hands = [hour, min] such that 
    the angle is target_angle degrees."""
    h, m = hands
    assert 0 < h <= 12 and 0 <= m < 60
    hour_angle = 30 * h + m / 2
    minute_angle = 6 * m
    return abs(hour_angle - minute_angle) in [target_angle, 360 - target_angle]
    return helper(8, 0, 2)

def g(target_angle=45):
    for h in range(1, 13):
        for m in range(60):
            hour_angle = 30 * h + m / 2
            minute_angle = 6 * m
            if abs(hour_angle - minute_angle) 
                return [h, m]
assert f(g()) == True

\end{python}
\caption{Example of programming problems and solutions from the P3 dataset \citep{schuster_programming_2021}. The problem function \texttt{f} verifies the solution provided in the first argument and returns a boolean, \texttt{True} if the solution is correct, \texttt{False} if not. A solution function \texttt{g} must return a valid solution such that \texttt{f(g()) == True}.}
\label{fig:example_programs}
\end{figure}
